# Supplementary material for: Non-Markovian escape under stochastic resetting
Source: arXiv:2509.11608 source file (2026-10-07)
Supplement: Supplementary file 1 [file SI.tex]

\documentclass[english,12pt,aps,pre,a4paper,preprintnumbers,floatfix,nofootinbib,showpacs,superscriptaddress,notitlepage]{revtex4-1}

\pdfoutput=1
\usepackage{subcaption}
\usepackage{graphicx}
\usepackage{rotate}
\usepackage[utf8]{inputenc}
\usepackage{bbold}
\usepackage{amsmath}
\usepackage{amssymb}
\usepackage{float}
\usepackage{comment}
\usepackage{soul}
\usepackage{lineno}
\usepackage[usenames,dvipsnames]{color}
\usepackage[colorinlistoftodos]{todonotes}
\usepackage[colorlinks=true, citecolor=blue, urlcolor=blue, linkcolor=blue]{hyperref}
\usepackage[normalem]{ulem}
\newcommand {\ignore}[1]{}
\usepackage{multirow}
\definecolor{darkred}{rgb}{0.6,0,0}
%%%%%%%%%%%%%%%%%%% Colours %%%%%%%%%%%%%%%%%%%

\newcommand{\bl}[1]{{\color{blue}  #1}}

%%%%%%%%%%%% Blind text for testing %%%%%%%%%%%
\usepackage[english]{babel}
\usepackage{blindtext}
%%%%%%%%%%%%%% Custom definitions %%%%%%%%%%%%%
\definecolor{midnightblue}{RGB}{25,25,112}
\definecolor{brown}{rgb}{0.59, 0.29, 0.0}

%

% \newcommand{\eps}{\varepsilon}
% \newcommand{\cm}{{cm}}
% \newcommand{\lab}{{lab}}
% \def\lfv{lepton flavour violation}

%\def\Q{\hbox{$\mathcal{Q }$}}

%%%%%%%%%%%%%%%%% Affiliations %%%%%%%%%%%%%%%%%
\newcommand{\AddrIISERchem}{Department of Chemistry, \\
Indian Institute of Science Education and Research (IISER) Bhopal \\
Bhopal Bypass Road, Bhauri, Bhopal 462066 INDIA}

\newcommand{\AddrIISERphy}{Department of Physics, \\
Indian Institute of Science Education and Research (IISER) Bhopal \\
Bhopal Bypass Road, Bhauri, Bhopal 462066 INDIA}

\begin{document}
% \linenumbers

%%%%%%%%%%%%%%% Title and authors %%%%%%%%%%%%%%%
% \title{Resetting causes memory loss: a transition from non-Markovian to Markovian dynamics}
\title{Supplementary Information for Non-Markovian escape under stochastic resetting}

\author{Debasish Saha} %\email{debashis21@iiserb.ac.in}
\affiliation{\AddrIISERphy}
\author{Rati Sharma}\email{rati@iiserb.ac.in}
\affiliation{\AddrIISERchem}

\maketitle

\section{Derivation of the Smoluchowski equation} 
\label{app:gle-to-fpe}
\noindent
The generalized Langevin equation (GLE) in the presence of fractional Gaussian noise (fGn) in the overdamped limit is given by \cite{mori1965, kubo1966, chaudhury2006}
\begin{equation}
\label{eq:gle}
    m\omega^{2} x(t) = -\zeta \int_{0}^{t} dt^{\prime} K(t-t^{\prime}) \dot{x}(t^{\prime}) + \theta(t)
\end{equation}
where $\theta(t)$ is the fGn, related to the friction kernel by the fluctuation-dissipation relation
%\begin{subequations}
\begin{equation}
\label{eq:fgn}
    \begin{split}
        \big\langle \theta(t)\theta(t^{\prime}) \big\rangle &= \xi k_{B}T K(t-t^{\prime}) \\
        K(t-t^{\prime}) &= 2H(2H - 1)|t-t^{\prime}|^{2H-2}
    \end{split}
\end{equation}
$K(t-t^{\prime})$ is the memory kernel that represents the temporal correlations of fluctuations giving rise to a non-Markovian process. $H$ is the Hurst index, which defines the strength of the correlation, typically varies within $\frac{1}{2} \leq H < 1$. $H=\frac{1}{2}$ represents the limiting case of Gaussian white noise (Markov process) where fluctuation is delta-correlated. Laplace transform (LT) of Eq. (\ref{eq:gle}) gives
\begin{equation}
\label{eq:LT}
    m\omega^{2} \hat{x}(s) = -\zeta \Big[\hat{K}(s) \big\{s\hat{x}(s) - x(0)\big\}\Big] + \hat{\theta}(s)
\end{equation}
Making some rearrangements, we get
\begin{equation}
\label{eq:LT_arrangement}
\hat{x}(s) = \frac{\zeta \hat{K}(s) x(0)}{s\zeta \hat{K}(s) + m\omega^{2}} + \frac{\hat{\theta}(s)}{s\zeta \hat{K}(s) + m\omega^{2}}
\end{equation}
Let us consider the following two functions:
\begin{subequations}
\label{eq:chi-and-phi}
\begin{equation}
    \label{eq:define_chi}
        \hat{\chi}(s) = \frac{\zeta \hat{K}(s)}{s\zeta \hat{K}(s) + m\omega^{2}}
    \end{equation}
    \begin{equation}
    \label{eq:define_phi}
        \hat{\phi}(s) = 1 - s\hat{\chi}(s) = \frac{m\omega^{2}}{s\zeta\hat{K}(s) + m\omega^{2}}
    \end{equation}
\end{subequations}
Using Eq. (\ref{eq:chi-and-phi}) in Eq. (\ref{eq:LT_arrangement}), we get
\begin{equation}
\label{eq:final_xs}
    \hat{x}(s) = x(0)\hat{\chi}(s) + \frac{1}{m\omega^{2}} \hat{\phi}(s) \hat{\theta}(s)
\end{equation}
Inverse Laplace transform of Eq. (\ref{eq:final_xs}) gives
\begin{equation}
\label{eq:xt_inverse_laplace}
    x(t) = x(0)\chi(t) + \frac{1}{m\omega^{2}} \int_{0}^{t} dt^{\prime} \phi(t-t^{\prime}) \theta(t^{\prime})
\end{equation}
From this we get
\begin{equation}
\label{eq:x0}
    x(0) = \frac{x(t)}{\chi(t)} - \frac{1}{m\omega^{2}\chi(t)} \int_{0}^{t} dt^{\prime} \phi(t-t^{\prime}) \theta(t^{\prime})
\end{equation}
Taking the first-order time derivative of Eq. (\ref{eq:xt_inverse_laplace}), and then using the expression of $x_{0}$, we get
\begin{equation}
\label{eq:x_dot}
\begin{split}
    \dot{x}(t) = \dot{\chi}(t)\bigg[\frac{x(t)}{\chi(t)} - \frac{1}{m\omega^{2}\chi(t)} \int_{0}^{t} dt^{\prime} \phi(t-t^{\prime}) \theta(t^{\prime}) \bigg] + \frac{1}{m\omega^{2}} \frac{d}{dt} \int_{0}^{t} dt^{\prime} \phi(t-t^{\prime}) \theta(t^{\prime})
\end{split}
\end{equation}
Now, let's do a simple differentiation,
\begin{equation}
\label{eq:derivative}
    \chi(t)\frac{d}{dt} \int_{0}^{t}dt^{\prime} \frac{\phi(t-t^{\prime})}{\chi(t)} \theta(t^{\prime})
    =-\frac{\dot{\chi}(t)}{\chi(t)} \int_{0}^{t}dt^{\prime} \phi(t-t^{\prime}) \theta(t^{\prime}) + \frac{d}{dt} \int_{0}^{t}dt^{\prime} \phi(t-t^{\prime}) \theta(t^{\prime})
\end{equation}
Using this, we can modify Eq. (\ref{eq:x_dot}) as 
\begin{equation}
\label{eq:x_dot}
\begin{split}
    \dot{x}(t) &= \frac{\dot{\chi}(t)}{\chi(t)}x(t) + \frac{1}{m\omega^{2}} \bigg[ -\frac{\dot{\chi}(t)}{\chi(t)} \int_{0}^{t} dt^{\prime} \phi(t-t^{\prime}) \theta(t^{\prime}) + \frac{d}{dt} \int_{0}^{t}dt^{\prime} \phi(t-t^{\prime}) \theta(t^{\prime}) \bigg] \\
    \dot{x}(t) &= \frac{\dot{\chi}(t)}{\chi(t)}x(t) + \frac{1}{m\omega^{2}} \chi(t)\frac{d}{dt} \int_{0}^{t} dt^{\prime} \frac{\phi(t-t^{\prime})}{\chi(t)} \theta(t^{\prime})
\end{split}
\end{equation}
Now, the probability $P(x,t)$ of finding the particle at $x$ at time $t$ is given by
\begin{equation}
\label{eq:prob_dist}
    P(x,t) = \big\langle \delta(x(t)-x) \big\rangle
\end{equation}
Taking time-derivative of Eq. (\ref{eq:prob_dist}), we get
\begin{equation}
\label{eq:prob_deriv}
\begin{split}
    \frac{\partial P(x,t)}{\partial t} =& \frac{\partial}{\partial t} \big\langle \delta(x(t)-x) \big\rangle 
    = \Big\langle \frac{\partial}{\partial x(t)}  \delta(x(t)-x) ~\dot{x}(t) \Big\rangle 
    = \Big\langle \frac{\partial}{\partial x(t)} \int_{0}^{\infty} dk e^{ik[x(t)-x]} ~\dot{x}(t) \Big\rangle \\
    = & \Big\langle \int_{0}^{\infty} dk e^{ik[x(t)-x]}(ik) ~\dot{x}(t) \Big\rangle 
    = \Big\langle -\frac{\partial}{\partial x} \int_{0}^{\infty} dk e^{ik[x(t)-x]} ~\dot{x}(t) \Big\rangle \\
    =& -\frac{\partial}{\partial x} \Big\langle \delta(x(t)-x) ~\dot{x}(t) \Big\rangle \\
\end{split}
\end{equation}
Now, putting $\dot{x}(t)$ from Eq. (\ref{eq:x_dot}) in Eq. (\ref{eq:prob_deriv}), we get
\begin{equation}
\label{eq:prob_deriv2}
\begin{split}
    \frac{\partial P(x,t)}{\partial t} = &-\frac{\partial}{\partial x} \Big\langle \delta(x(t)-x) \frac{\dot{\chi}(t)}{\chi(t)}x(t) \Big\rangle - \frac{\partial}{\partial x} \Big\langle \delta(x(t)-x) \frac{1}{m\omega^{2}} \chi(t)\frac{d}{dt} \int_{0}^{t} dt^{\prime} \frac{\phi(t-t^{\prime})}{\chi(t)} \theta(t^{\prime}) \Big\rangle
\end{split}
\end{equation}
The first term in the RHS of Eq. (\ref{eq:prob_deriv2}) can be solved as
\begin{equation}
\label{eq:1st_term}
\begin{split}
    -\frac{\partial}{\partial x} \Big\langle \delta(x(t)-x) \frac{\dot{\chi}(t)}{\chi(t)}~x(t) \Big\rangle 
    = \eta(t) \frac{\partial}{\partial x} \Big\langle \delta(x(t)-x) ~x(t) \Big\rangle
    = \eta(t) \frac{\partial}{\partial x} xP(x,t) 
\end{split}
\end{equation}
Considering $\eta(t) = -\dot{\chi}(t)/\chi(t)$, and using the identity $\delta(x-a)f(x) = \delta(x-a)f(a)$.
\\~\\
The second term in the RHS of Eq. (\ref{eq:prob_deriv2}) can be written as
\begin{equation}
\label{eq:2nd_term}
\begin{split}
    & -\frac{\partial}{\partial x}\Big\langle \delta(x(t)-x) \frac{1}{m\omega^{2}} ~\chi(t)\frac{d}{dt} \int_{0}^{t} dt^{\prime} \frac{\phi(t-t^{\prime})}{\chi(t)} \theta(t^{\prime}) \Big\rangle \\
    =& -\frac{1}{m\omega^{2}} \frac{\partial}{\partial x}\Big\langle \delta(x(t)-x) ~\chi(t)\frac{d}{dt} \int_{0}^{t} dt^{\prime} \frac{\phi(t-t^{\prime})}{\chi(t)} \theta(t^{\prime}) \Big\rangle 
    = -\frac{1}{m\omega^{2}} \frac{\partial}{\partial x}\Big\langle \delta(x(t)-x) ~\hat{\theta}(t) \Big\rangle 
\end{split}
\end{equation}
considering, \[ \hat{\theta}(t) = \chi(t)\frac{d}{dt} \int_{0}^{t} dt^{\prime} ~\frac{\phi(t-t^{\prime})}{\chi(t)} ~\theta(t^{\prime}) \]
Using Eq. (\ref{eq:1st_term}) and (\ref{eq:2nd_term}) in Eq. (\ref{eq:prob_deriv2}), we can write
\begin{equation}
\label{eq:prob_deriv3}
    \frac{\partial P(x,t)}{\partial t} = \eta(t)\frac{\partial}{\partial x}xP(x,t) - \frac{1}{m\omega^{2}}\frac{\partial}{\partial x} \Big\langle \delta(x(t) - x) ~\hat{\theta}(t) \Big\rangle
\end{equation}
Novikov’s theorem \cite{novikov1965} states
\begin{equation}
\label{eq:2nd_term_of_fpe}
\begin{split}
    \big\langle \delta(x(t) -x)\hat{\theta}(t) \big\rangle
    = & \int_{0}^{t}dt^{\prime} \big\langle \hat{\theta}(t) \hat{\theta}(t^{\prime})\big\rangle \Big\langle\frac{\delta}{\delta\hat{\theta}(t^{\prime})}\delta\big(x(t) - x\big) \Big\rangle \\
    = & \int_{0}^{t}dt^{\prime} \big\langle \hat{\theta}(t) \hat{\theta}(t^{\prime})\big\rangle \Big\langle\frac{\delta}{\delta x(t)}\delta\big(x(t) - x\big) \frac{\delta x(t)}{\delta\hat{\theta}(t^{\prime})} \Big\rangle \\
    = & -\frac{\partial}{\partial x}\int_{0}^{t}dt^{\prime} \big\langle \hat{\theta}(t) \hat{\theta}(t^{\prime})\big\rangle \Big\langle \delta\big(x(t) - x\big) \frac{\delta x(t)}{\delta\hat{\theta}(t^{\prime})} \Big\rangle
\end{split}
\end{equation}
Eq. (\ref{eq:x_dot}) can be rewritten as
\begin{equation}
\label{eq:diff_eq}
\begin{split}
    \dot{x}(t) - \eta(t)x(t) &= \frac{1}{m\omega^{2}} \chi(t)\frac{d}{dt} \int_{0}^{t}dt^{\prime} \frac{\phi(t-t^{\prime})}{\chi(t)} \theta(t^{\prime}) 
    = \frac{1}{m\omega^{2}} \hat{\theta}(t) \\
    \dot{x}(t) - \eta(t)x(t) &= M(t)
\end{split}
\end{equation}
where, $M(t) = \frac{1}{m\omega^{2}} \hat{\theta}(t)$. Eq. (\ref{eq:diff_eq}) is a linear first-order differential equation which can be solved using the integrating factor as follows
\begin{equation}
\begin{split}
    & x(t)\exp{\Big(-\int_{0}^{t} \eta(t^{\prime}) dt^{\prime}\Big)} - x(0) = \int_{0}^{t} dt^{\prime} \exp{\Big(-\int_{0}^{t^{\prime}} dt^{\prime\prime}\eta(t^{\prime})\Big)} M(t^{\prime}) \\
    & x(t) = \exp{\Big(\int_{0}^{t} \eta(t^{\prime}) dt^{\prime}\Big)} \bigg[x(0) + \frac{1}{m\omega^{2}} \int_{0}^{t} dt^{\prime} \exp{ \Big( -\int_{0}^{t^{\prime}} dt^{\prime\prime}\eta(t^{\prime\prime})\Big)} \hat{\theta}(t^{\prime}) \bigg] \\
\end{split}
\end{equation}
The fractional derivative in Eq (\ref{eq:2nd_term_of_fpe}) can be evaluated as 
\begin{equation}
\begin{split}
    \frac{\delta x(t)}{\delta \hat{\theta}(t^{\prime})} &= \frac{\delta}{\delta \hat{\theta}(t^{\prime})} \bigg[ \exp{\Big(\int_{0}^{t} \eta(t^{\prime}) dt^{\prime}\Big)} \bigg\{x(0) + \frac{1}{m\omega^{2}} \int_{0}^{t} dt^{\prime} \exp{\Big(-\int_{0}^{t^{\prime}} dt^{\prime\prime}\eta(t^{\prime\prime})\Big)} \hat{\theta}(t^{\prime}) \bigg\} \bigg] \\
    &= \exp{\Big(\int_{0}^{t}dt^{\prime}\eta(t^{\prime})\Big)} \bigg[\frac{1}{m\omega^{2}}\int_{0}^{t} dt^{\prime} \exp{\Big(-\int_{0}^{t^{\prime}}dt^{\prime\prime}\eta(t^{\prime\prime})\Big)} \frac{\delta\hat{\theta}(t^{\prime})}{\delta\hat{\theta}(t^{\prime\prime})} \bigg] \\
    &= \exp{\Big(\int_{0}^{t}dt^{\prime}\eta(t^{\prime})\Big)} \bigg[\frac{1}{m\omega^{2}}\int_{0}^{t} dt^{\prime} \exp{\Big(-\int_{0}^{t^{\prime}}dt^{\prime\prime}\eta(t^{\prime\prime})\Big)} \delta\big(\hat{\theta}(t^{\prime}) - \hat{\theta}(t^{\prime\prime})\big) \bigg] \\
    &= \exp{\Big(\int_{0}^{t}dt^{\prime}\eta(t^{\prime})\Big)} \bigg[\frac{1}{m\omega^{2}} \exp{\Big(-\int_{0}^{t^{\prime}}dt^{\prime\prime}\eta(t^{\prime\prime})\Big)} \bigg] \\
    &= \frac{1}{m\omega^{2}} \exp{\Big(\int_{0}^{t}dt^{\prime}\eta(t^{\prime}) -\int_{0}^{t^{\prime}}dt^{\prime}\eta(t^{\prime})\Big)} \\
    &= \frac{1}{m\omega^{2}} \exp{\Big(-\int_{t}^{0}dt^{\prime}\eta(t^{\prime}) -\int_{0}^{t^{\prime}}dt^{\prime}\eta(t^{\prime})\Big)} \\
    &= \frac{1}{m\omega^{2}} \exp{\Big(-\int_{t}^{t^{\prime}}dt_{1}\eta(t_{1})} \Big) \\
\end{split}
\end{equation}
Combining all terms in one place, we get
\begin{equation}
\label{eq:fpe}
\begin{split}
    \frac{\partial P(x,t)}{\partial t} &= \eta(t) \frac{\partial}{\partial x} xP(x,t) - \frac{1}{m\omega^{2}} \frac{\partial}{\partial x} \Big\langle \delta\big( x(t) - x)\Big\rangle \\
    &= \eta(t) \frac{\partial}{\partial x} xP(x,t) - \frac{1}{m\omega^{2}} \frac{\partial}{\partial x} \bigg[ -\frac{\partial}{\partial x} \int_{0}^{t}dt^{\prime} \big\langle \hat{\theta}(t) \hat{\theta}(t^{\prime}) \big\rangle \\
    & \hspace{5cm} \times \bigg\langle \delta(x(t) - x) \frac{1}{m\omega^{2}} \exp{\bigg(-\int_{t}^{t^{\prime}}}dt_{1}\eta(t_{1}) \bigg) \bigg\rangle \bigg] \\
    &= \eta(t) \frac{\partial}{\partial x} x P(x,t) + \frac{1}{m^{2}\omega^{4}} \frac{\partial^{2}}{\partial x^{2}} \big\langle\delta(x(t) - x)\big\rangle \int_{0}^{t}dt^{\prime} \big\langle \hat{\theta}(t) \hat{\theta}(t^{\prime}) \big\rangle \exp{\bigg(-\int_{t}^{t^{\prime}}}dt_{1}\eta(t_{1}) \bigg) \\
    &= \eta(t) \frac{\partial}{\partial x} xP(x,t) + \frac{1}{m^{2}\omega^{4}} \frac{\partial^{2}}{\partial x^{2}} P(x,t) D(t) 
\end{split}
\end{equation}
where,
\begin{equation}
\label{eq:dt1}
\begin{split}
    D(t) &= \int_{0}^{t}dt^{\prime} \big\langle \hat{\theta}(t) \hat{\theta}(t^{\prime}) \big\rangle \exp{\bigg(-\int_{t}^{t^{\prime}}}dt_{1}\eta(t_{1}) \bigg) \\
    &= \int_{0}^{t} dt^{\prime} \Big\langle \chi(t)\frac{d}{dt} \int_{0}^{t}dt_{1} \frac{\phi(t-t_{1})}{\chi(t)} \theta(t_{1}) ~\chi(t^{\prime})\frac{d}{dt^{\prime}} \int_{0}^{t^{\prime}}dt_{2} \frac{\phi(t^{\prime}-t_{2})}{\chi(t^{\prime})} \theta(t_{2}) \Big\rangle ~\frac{\chi(t^{\prime})}{\chi(t)}
\end{split}
\end{equation}
by doing the integration 
\[
\exp\bigg( -\int_{t}^{t^{\prime}} dt_{1}\eta(t_{1})\bigg) 
= \exp\bigg(\int_{t}^{t^{\prime}} dt_{1} \frac{\dot{\chi}(t_{1})}{\chi(t_{1})} \bigg)
= \exp\bigg(\int_{t}^{t^{\prime}} \frac{d\big(\chi(t_{1})\big)}{\chi(t_{1})} \bigg)
= \exp\bigg(\ln{\frac{\chi(t^{\prime})}{\chi(t)}} \bigg)
= \frac{\chi(t^{\prime})}{\chi(t)}
\]
Now, Eq. (\ref{eq:dt1}) can be simplified to
\begin{equation}
\label{eq:dt2}
\begin{split}
    D(t) &= \int_{0}^{t}dt^{\prime} \chi(t)\frac{d}{dt} \int_{0}^{t}dt_{1} \frac{\phi(t-t_{1})}{\chi(t)} ~\chi(t^{\prime})\frac{d}{dt^{\prime}} \int_{0}^{t^{\prime}}dt_{2} \frac{\phi(t^{\prime}-t_{2})}{\chi(t^{\prime})} \big\langle \theta(t_{1})\theta(t_{2}) \big\rangle \frac{\chi(t^{\prime})}{\chi(t)} \\
    % &= \chi(t) \int_{0}^{t} dt_{2} \phi(t-t_{2}) \frac{d}{dt} \int_{0}^{t^{\prime}}dt_{1} \frac{\phi(t-t_{1})}{\chi(t)} \big\langle \theta(t_{1})\theta(t_{2}) \big\rangle
\end{split}
\end{equation}
We can write,
\[
\chi^{2}(t) \frac{d}{dt} \frac{1}{\chi^{2}(t)} = 2 \chi(t) \frac{d}{dt} \frac{1}{\chi(t)}
\]
using which, we can rewrite Eq. (\ref{eq:dt2}) as
\begin{equation}
\label{eq:dt3}
    D(t) = \frac{1}{2}\chi^{2}(t) \frac{d}{dt} \frac{1}{\chi^{2}(t)} \int_{0}^{t}dt_{1}\int_{0}^{t}dt_{2} ~\phi(t-t_{1}) \phi(t-t_{2}) \big\langle \theta(t_{1})\theta(t_{2}) \big\rangle
\end{equation}
Now, let us solve Eq. (\ref{eq:dt3}) explicitly to get $D(t)$, which can be done as follows. We consider,
\begin{equation}
\label{eq:final_int}
    I = \int_{0}^{t}dt_{1}\int_{0}^{t}dt_{2} ~\phi(t-t_{1}) \phi(t-t_{2}) \big\langle \theta(t_{1})\theta(t_{2}) \big\rangle
\end{equation}
where, $\big\langle \theta(t_{1})\theta(t_{2}) \big\rangle = \zeta k_{B}TK(t_{1}-t_{2})$. Using this in Eq. (\ref{eq:final_int}), we can write 
\begin{equation}
\label{eq:final_int2}
    I = \zeta k_{B}T \int_{0}^{t}dt_{1}\int_{0}^{t}dt_{2} ~\phi(t-t_{1}) \phi(t-t_{2}) K(t_{1}-t_{2})
\end{equation}
Laplace transform (LT) of Eq. (\ref{eq:final_int}) gives,
\begin{equation}
\label{eq:final_int2_lt}
\begin{split}
    I^{\prime} &= \zeta k_{B}T \int_{0}^{\infty}dt~ e^{-z_{1}t} \int_{0}^{\infty} dt~ e^{-z_{2}t} \int_{0}^{t}dt_{1} \int_{0}^{t}dt_{2} ~\phi(t-t_{1}) \phi(t-t_{2}) K(t_{1}-t_{2}) \\
    &= \zeta k_{B}T \int_{0}^{\infty}dt \int_{0}^{\infty} dt~ e^{-z_{1}t} e^{-z_{2}t} \int_{0}^{t}dt_{1} \int_{0}^{t}dt_{2} ~\phi(t-t_{1}) \phi(t-t_{2}) K(t_{1}-t_{2}) \\
    &= \zeta k_{B}T \int_{0}^{\infty}dt \int_{0}^{\infty} dt~ \int_{0}^{\infty}dt_{1} \int_{0}^{\infty}dt_{2} ~ H(t-t_{1})~ H(t-t_{2}) \\
    & \hspace{5cm} \times e^{-z_{1}t} e^{-z_{2}t} ~\phi(t-t_{1}) \phi(t-t_{2}) K(t_{1}-t_{2}) \\
    &= \zeta k_{B}T \int_{0}^{\infty}dt_{1} \int_{0}^{\infty}dt_{2} \int_{t_{1}}^{\infty}dt \int_{t_{2}}^{\infty} dt ~e^{-z_{1}t} e^{-z_{2}t} ~\phi(t-t_{1}) \phi(t-t_{2}) K(t_{1}-t_{2}) \\
    &= \zeta k_{B}T \int_{0}^{\infty}dt_{1} \int_{t_{1}}^{\infty}dt \int_{0}^{\infty}dt_{2} \int_{t_{2}}^{\infty} dt ~e^{-z_{1}(t-t_{1})} e^{-z_{2}(t-t_{2})} ~e^{-z_{1}t_{1}} e^{-z_{2}t_{2}} \\
    & \hspace{7cm} \times \phi(t-t_{1}) \phi(t-t_{2}) K(t_{1}-t_{2})
\end{split}
\end{equation}
$H(x-a)$ is the Heaviside theta function. Now, consider $t-t_{1} = x$ with $x\in [0,\infty]$ and $t-t_{2} = y$ with $y\in [0,\infty]$. Substituting these, we can rewrite Eq. (\ref{eq:final_int2_lt}) as
\begin{equation}
\label{eq:final_int2_lt2}
\begin{split}
    I^{\prime} &= \zeta k_{B}T \int_{0}^{\infty}dt_{2} \int_{0}^{\infty}dy \int_{0}^{\infty}dt_{1} \int_{0}^{\infty} dx ~e^{-z_{2}y} e^{-z_{1}x} ~e^{-z_{2}t_{2}} e^{-z_{1}t_{1}} \phi(x) \phi(y) K(t_{1}-t_{2}) \\
    &= \zeta k_{B}T \int_{0}^{\infty}dt_{2} ~e^{-z_{2}t_{2}} \bigg[\int_{0}^{\infty}dy ~e^{-z_{2}y} \phi(y) \bigg] \int_{0}^{\infty}dt_{1} e^{-z_{1}t_{1}} \bigg[ \int_{0}^{\infty} dx  e^{-z_{1}x}  \phi(x) \bigg] K(t_{1}-t_{2}) \\
    &= \zeta k_{B}T ~\hat{\phi}(z_{1}) \hat{\phi}(z_{2}) \int_{0}^{\infty} dt_{2} \int_{0}^{\infty} dt_{1} ~e^{-z_{2}t_{2}} e^{-z_{1}t_{1}} K(t_{1}-t_{2})
\end{split}
\end{equation}
We are considering the absolute time difference in the memory kernel, \emph{i.e.}, $K(t_{1}-t_{2}) \propto |t_{1}-t_{2}|$. Therefore, two cases may appear, either $t_{1} > t_{2}$, or $t_{1} < t_{2}$. Considering both of them, one can get
\begin{equation}
\label{eq:final_int2_lt3}
\begin{split}
    &\int_{0}^{\infty} dt_{2} \int_{0}^{\infty} dt_{1} ~e^{-z_{2}t_{2}} e^{-z_{1}t_{1}} K(t_{1}-t_{2}) \\
    =& \int_{0}^{\infty} dt_{2} \int_{0}^{t_{2}} dt_{1} ~e^{-z_{2}t_{2}} e^{-z_{1}t_{1}} K(t_{1}-t_{2}) + \int_{0}^{\infty} dt_{2} \int_{t_{2}}^{\infty} dt_{1} ~e^{-z_{2}t_{2}} e^{-z_{1}t_{1}} K(t_{2}-t_{1}) \\
    =& \int_{0}^{\infty} dt_{2} \int_{0}^{t_{2}} dt_{1} ~e^{-z_{1}(t_{1}-t_{2})} e^{-(z_{1}+z_{2})t_{2}} K(t_{1}-t_{2}) \\ &\hspace{3cm}+ \int_{0}^{\infty} dt_{2} \int_{t_{2}}^{\infty} dt_{1} ~e^{-z_{1}(t_{1}-t_{2})} e^{-(z_{1}+z_{2})t_{2}} K(t_{2}-t_{1}) \\
    =& ~ A_{1} + A_{2}
\end{split}
\end{equation}
Now consider $t_{1}-t_{2} = p$ with $p\in[-t_{2},0]$ for the first integration and $p\in[0,\infty]$ for the second integration. Performing the first integration $A_{1}$, using these substitutions, we obtain
\begin{equation}
\label{eq:a1}
\begin{split}
    A_{1} &= \int_{0}^{\infty}dt_{2} \int_{0}^{t_{2}}dp ~e^{-z_{1}p} e^{-(z_{1}+z_{2})t_{2}} K(p) \\
    &= \int_{0}^{\infty}dt_{2} \int_{0}^{\infty}dp ~H(t_{2}-p) ~e^{-z_{1}p} e^{-(z_{1}+z_{2})t_{2}} K(p) \\
    &= \int_{0}^{\infty}dp ~e^{-z_{1}p} K(p) \int_{0}^{\infty}dt_{2} ~H(t_{2}-p) e^{-(z_{1}+z_{2})t_{2}} \\
    &= \int_{0}^{\infty}dp ~e^{-z_{1}p} K(p) \int_{p}^{\infty}dt_{2} ~e^{-(z_{1}+z_{2})(t_{2}-p)} \\
    &= \int_{0}^{\infty}dp ~e^{-z_{1}p} K(p) \int_{p}^{\infty}dt_{2} ~e^{-(z_{1}+z_{2})t_{2}} ~e^{z_{1}p} ~e^{z_{2}p} \\
    &= \int_{0}^{\infty}dp ~e^{z_{2}p} K(p) \int_{p}^{\infty}dt_{2} ~e^{-(z_{1}+z_{2})t_{2}} 
    = \int_{0}^{\infty}dp ~e^{z_{2}p} K(p) \bigg[ \frac{e^{-(z_{1}+z_{2})t_{2}}}{z_{1}+z_{2}} \bigg] \\
    &= \frac{1}{z_{1}+z_{2}} \int_{0}^{\infty}dp ~e^{-z_{1}p} ~K(p)
    = \frac{\hat{K}(z_{1})}{z_{1}+z_{2}}
\end{split}
\end{equation}
Similarly, we can show 
\begin{equation}
\label{eq:a2}
    A_{2} = \frac{\hat{K}(z_{2})}{z_{1}+z_{2}}
\end{equation}
Using Eq. (\ref{eq:final_int2_lt3}), (\ref{eq:a1}) and (\ref{eq:a2}) in Eq. (\ref{eq:final_int2_lt2}), we get \cite{pottier2003}
\begin{equation}
\label{eq:final_int2_lt4}
\begin{split}
    I^{\prime} &= \zeta k_{B}T ~\hat{\phi}(z_{1}) \hat{\phi}(z_{2}) \bigg[ \frac{\hat{K}(z_{1}) + \hat{K}(z_{1})}{z_{1}+z_{2}} \bigg] \\
    &= \frac{\zeta k_{B}T}{z_{1}+z_{2}} \bigg[ \hat{\phi}(z_{1}) \hat{\phi}(z_{2}) \hat{K}(z_{1}) + \hat{\phi}(z_{1}) \hat{\phi}(z_{2}) \hat{K}(z_{2}) \bigg]
\end{split}
\end{equation}
Eq. (\ref{eq:chi-and-phi}) can be rewritten in terms of variable $z$ as
\begin{equation}
\begin{split}
    & \hat{\phi}(z) = 1 - z\hat{\chi}(z) 
    = 1 - \frac{z\zeta \hat{K}(z)}{z\zeta \hat{K}(z) +m\omega^{2}}
    =\frac{m\omega^{2}}{m\omega^{2} + z\zeta \hat{K}(z)} \\
    & m\omega^{2} ~\hat{\phi}(z) + z\zeta \hat{\phi}(z) \hat{K}(z) = m\omega^{2} \\
    & z\zeta \hat{\phi}(z) \hat{K}(z) = m\omega^{2} - m\omega^{2} ~\hat{\phi}(z) \\
    & \hat{\phi}(z) \hat{K}(z)
     = \frac{m\omega^{2}}{\zeta} ~\frac{1 - \hat{\phi}(z)}{z}
     = \frac{m\omega^{2}}{\zeta} ~\frac{1 - 1 + z\hat{\chi}(z)}{z}
     = \frac{m\omega^{2}}{\zeta} ~\hat{\chi}(z)
\end{split}
\end{equation}
Therefore, Eq. (\ref{eq:final_int2_lt4}) becomes
\begin{equation}
\label{eq:final_int2_lt5}
\begin{split}
    I^{\prime} &= \frac{\zeta k_{B}T}{z_{1}+z_{2}} \bigg[ \frac{m\omega^{2}}{\zeta} ~\hat{\chi}(z_{1}) \hat{\phi}(z_{2}) + \frac{m\omega^{2}}{\zeta} ~\hat{\chi}(z_{2}) \hat{\phi}(z_{1}) \bigg] \\
    &= \frac{m\omega^{2} k_{B}T}{z_{1}+z_{2}} \bigg[\hat{\chi}(z_{1}) \Big(1 - z_{2}\hat{\chi}(z_{2})\Big) + \hat{\chi}(z_{2}) \Big(1 - z_{1}\hat{\chi}(z_{1})\Big) \bigg] \\
    &= \frac{m\omega^{2} k_{B}T}{z_{1}+z_{2}} \bigg[\hat{\chi}(z_{1}) - z_{2}\hat{\chi}(z_{1})\hat{\chi}(z_{2}) + \hat{\chi}(z_{2}) - z_{1}\hat{\chi}(z_{2})\hat{\chi}(z_{1}) \bigg] \\
    &= \frac{m\omega^{2} k_{B}T}{z_{1}+z_{2}} \bigg[\hat{\chi}(z_{1}) + \hat{\chi}(z_{2}) - (z_{1}+z_{2}) \hat{\chi}(z_{2})\hat{\chi}(z_{1}) \bigg] \\
    &= m\omega^{2} k_{B}T \bigg[ \frac{\hat{\chi}(z_{1}) + \hat{\chi}(z_{2})}{z_{1}+z_{2}} - \hat{\chi}(z_{1})\hat{\chi}(z_{2}) \bigg] \\
\end{split}
\end{equation}
Inverse LT of Eq. (\ref{eq:final_int2_lt5}) gives
\begin{equation}
\label{eq:inverse_lt}
\begin{split}
    I &= m\omega^{2} k_{B}T \int_{0}^{\infty}dz_{1} \int_{0}^{\infty}dz_{2} ~e^{z_{1}t} e^{z_{2}t} \bigg[ \frac{\hat{\chi}(z_{1}) + \hat{\chi}(z_{2})}{z_{1}+z_{2}} - \hat{\chi}(z_{1})\hat{\chi}(z_{2})\bigg] \\
    &= m\omega^{2} k_{B}T \Big[ \chi(0) - \chi^{2}(t) \Big] 
    = m\omega^{2} k_{B}T \Big[ 1 - \chi^{2}(t) \Big]
\end{split}
\end{equation}
We can finally write Eq. (\ref{eq:dt3}) as
\begin{equation}
\begin{split}
    D(t) &= \frac{1}{2} \chi^{2}(t)\frac{d}{dt} \frac{1}{\chi^{2}(t)} m\omega^{2} k_{B}T \Big[ 1 - \chi^{2}(t) \Big] 
    = \frac{1}{2}m\omega^{2} k_{B}T ~\chi^{2}(t)\frac{d}{dt} \Big[ \frac{1}{\chi^{2}(t)} - 1 \Big] \\ 
    &= -m\omega^{2} k_{B}T ~\frac{\dot{\chi}(t)}{\chi(t)} 
    = m\omega^{2} k_{B}T ~\eta(t)
\end{split}
\end{equation}
Therefore, the equation of probability density as mentioned in Eq. (\ref{eq:fpe}) can be expressed as
\begin{equation}
    \frac{\partial P(x,t)}{\partial t} = \eta(t) \frac{\partial}{\partial x} x P(x,t) + \frac{1}{m^{2}\omega^{4}} \frac{\partial^{2}}{\partial x^{2}} P(x,t) ~m\omega^{2} k_{B}T ~\eta(t)
\end{equation}
\begin{equation}
    \frac{\partial P(x,t)}{\partial t} = \eta(t) \frac{\partial}{\partial x} x P(x,t) + \eta(t) \frac{k_{B}T}{m\omega^{2}} \frac{\partial^{2}}{\partial x^{2}} P(x,t)
\end{equation}
This is the well-known Smoluchowski equation representing the dynamics of a particle diffusing under a harmonic trap in a non-Markovian environment and under the influence of fractional Gaussian noise.

\section{Derivation of the propagator $G(x, t|x_{0}, t_{0})$} 
\label{app:fpe-to-green-function}
\noindent
In this section, we will derive the Green's function from the FPE. This is a generic approach, and valid for both Markovian and non-Markovian systems. We start with the FPE, as we mentioned in Eq. (\bl{3}), and derived in Section \ref{app:gle-to-fpe} is
\begin{equation}
    \frac{\partial P(x,t)}{\partial t} = \eta(t) \bigg[\frac{\partial}{\partial x} x + \frac{k_{B}T}{m\omega^{2}} \frac{\partial^{2}}{\partial x^{2}} \bigg]P(x,t)
\end{equation}
The equivalent equation for the Green's function is
\begin{equation}
\label{eq:eqv-greens}
    \frac{\partial}{\partial t} G(x,t|x_{0},t_{0}) = \mathbf{L} G(x,t|x_{0},t_{0})
\end{equation}
corresponding to the initial conditions:
\begin{equation}
    G(x,t|x_{0},0) = \delta(x-x_{0}) \delta(t)
\end{equation}
Here $\mathbf{L}$ is the Fokker-Planck operator defined as follows,
\begin{equation}
    \mathbf{L} = \eta(t) \bigg[\frac{\partial}{\partial x} x + \frac{k_{B}T}{m\omega^{2}} \frac{\partial^{2}}{\partial x^{2}} \bigg]
\end{equation}
The Fourier transform of Green's function is
\begin{equation}
    \hat{G}(k,t|x_{0},0) = \frac{1}{2\pi} \int_{-\infty}^{\infty} dk ~e^{ikx} G(x,t|x_{0},0)
\end{equation}
Carrying out the Fourier transform of Eq. (\ref{eq:eqv-greens}), we get
\begin{equation}
    \frac{\partial}{\partial t} \hat{G}(k,t|x_{0},0) = \bigg[ \eta(t) - \eta(t)k \frac{\partial}{\partial k} - \eta(t) \frac{k_{B}T}{m\omega^{2}}k^{2} \bigg] \hat{G}(k,t|x_{0},0)
\end{equation}
Dividing both sides by $\hat{G}(k,t|x_{0},0)$, we get
\begin{equation}
\label{eq:log-green-func}
    \frac{\partial}{\partial t} \ln{\hat{G}(k,t|x_{0},0)} = \eta(t) - \eta(t)k \frac{\partial}{\partial k} \ln{\hat{G}(k,t|x_{0},0)} - \eta(t) \frac{k_{B}T}{m\omega^{2}}k^{2} 
\end{equation}
Now, consider the Gaussian ansatz:
\begin{equation}
\label{eq:gaussian-ansatz}
    \ln{\hat{G}(k,t|x_{0},0)} = ika(t) - \frac{1}{2} k^{2} b(t)
\end{equation}
Taking the time derivative of Eq. (\ref{eq:gaussian-ansatz}), and comparing the coefficients of $k$ and $k^{2}$ with the same in Eq. (\ref{eq:log-green-func}), we get
\begin{equation}
\begin{split}
    \frac{d}{dt} a(t) &= -\eta(t) a(t) \\
    \frac{d}{dt} b(t) &= -2\eta(t) \bigg( b(t) - \frac{k_{B}T}{m\omega^{2}} \bigg)
\end{split}
\end{equation}
with the initial conditions: $a(0) = x_{0}$ and $b(0) = 0$. Solutions of these two equations are,
\begin{equation}
\begin{split}
    a(t) &= \chi(t) x_{0} \\
    b(t) &= \frac{k_{B}T}{m\omega^{2}} \Big( 1 - \chi^{2}(t) \Big)
\end{split}
\end{equation}
Now, taking the inverse Fourier transform of Eq. (\ref{eq:gaussian-ansatz}), we get
\begin{equation}
\label{eq:gaussian-inverse-fourier}
    G(x,t|x_{0},0) = \sqrt{\frac{1}{2\pi b(t)}} \exp{\Bigg[\frac{-\big(x-a(t)\big)^{2}}{2b(t)} \Bigg]}
\end{equation}
Finally, putting the values of $a(t)$ and $b(t)$, we get
\begin{equation}
\label{eq:final-green-function}
    G(x,t|x_{0},0) = \sqrt{\frac{m\omega^{2}}{2\pi k_{B}T \big(1-\chi^{2}(t)\big)}} \exp{\Bigg[-\frac{m\omega^{2}\big(x-x_{0}\chi(t)\big)^{2}}{2 k_{B}T \big(1-\chi^{2}(t)\big)} \Bigg]}
\end{equation}
This is the desired Green's function as mentioned in the main text. This equation has been used in the renewal equation to compute position distributions and related properties under resetting.

\section{Calculation of $\chi(t) = E_{b}\big[-(t/\tau_{0})^{b}\big]$} 
\label{app:derive-chi}
\noindent
The definition of $\hat{\chi}(s)$ in terms of Laplace variable $s$ is
\begin{equation}
\label{eq:chi_s}
    \hat{\chi}(s) = \frac{\zeta \hat{K}(s)}{s\zeta \hat{K}(s) + m\omega^{2}}
\end{equation}
$\hat{K}(s)$ is the LT of the function $K(t-t^{\prime}) = 2H(2H-1)|t-t^{\prime}|^{2H-2}$. Taking LT of this, we get
\begin{equation}
    \hat{K}(s) = \Gamma(2H+1) ~s^{1-2H}
\end{equation}
Using this expression, we can rewrite Eq. (\ref{eq:chi_s}) as following:
\begin{equation}
    \hat{\chi}(s) = \frac{\zeta \Gamma(2H+1) s^{1-2H}}{\zeta \Gamma(2H+1) ~s^{2-2H} + m\omega^{2}}
\end{equation}
Now, the LT of the Mittage-Leffler function is
\begin{equation}
\label{eq:laplace-mittag-leffler}
    \mathcal{L}\Big[ E_{\alpha}\big(-a t^{\alpha}\big) \Big] (s) = \frac{s^{\alpha-1}}{s^{\alpha} + a}
\end{equation}
Taking the inverse LT of Eq. (\ref{eq:laplace-mittag-leffler}), and comparing the coefficients, we finally obtain
\begin{equation}
    \chi(t) = E_{b} \Big[-(t/\tau_{0})^{b} \Big]
\end{equation}
where, $b = 2-2H$ and $\tau_{0} = \big[\zeta \Gamma(2H+1)/m\omega^{2} \big]^{1/b}$.

\bibliographystyle{unsrt}
\bibliography{references}

\end{document}
